# Supplementary material for: Backstepping Reach-avoid Controller Synthesis for Multi-input Multi-output Systems with Mixed Relative Degrees
Source: arXiv:2505.03612 source file (2025-05-06)
Supplement: Supplementary file 1 [file appendix.tex]

\section{Appendix}

\subsection{Proof of Theorem 2}

Given 
\begin{align*}
    \psi_{\gamma}(\bm{y}) = \psi(\bm{y}) - \sum_{l=1}^{\gamma-1}\frac{1}{2\mu_{l}}\|\eta_{l+1}-k_{l}(z_{l})\|_{2}^{2}
\end{align*}
Let 
\begin{align*}
    F &= L_f^\gamma h(x) \\
    G &= 
    \begin{bmatrix}
        L_{g_1}(L_f^{\gamma-1}h(x)) & \cdots & L_{g_m}(L_f^{\gamma-1}h(x))
    \end{bmatrix}
\end{align*}
Take the derivative of $\psi_\gamma$ with respect to time,
\begin{align*}
    \dot{\psi_\gamma}(\bm{y}) =& (\frac{\partial \psi(y)}{\partial \bm{y}})^\top \dot{y} \\
    &- \sum_{l=1}^{\gamma-1} \frac{(\eta_{l+1} - k_l)^\top}{\mu_l} (\dot{\eta}_{l+1} - \sum_{s=1}^l \frac{\partial k_l}{\partial \eta_s} \dot{\eta}_s) \\
    =& (\frac{\partial \psi(y)}{\partial \bm{y}})^\top  (\eta_2 -k_1 + k_1) \\
    &- \frac{(\eta_2 - k_1)^\top}{\mu_1}(\eta_3 - k_2 + k_2 - \sum_{s=1}^1 \frac{\partial k_1}{\partial \eta_s} \dot{\eta}_s) \\
    &- \frac{(\eta_3 - k_2)^\top}{\mu_2}(\eta_4 - k_3 + k_3 - \sum_{s=1}^2 \frac{\partial k_2}{\partial \eta_s} \dot{\eta}_s) \\
    &\cdots \\
    &- \frac{(\eta_{\gamma-2} - k_{\gamma-3})^\top}{\mu_{\gamma-3}} (\eta_{\gamma-1} - k_{\gamma-2} + k_{\gamma-2} \\ &\qquad \qquad \qquad \qquad \qquad \quad - \sum_{s=1}^{\gamma-3} \frac{\partial k_{\gamma-3}}{\partial \eta_s} \dot{\eta}_s) \\
    &- \frac{(\eta_{\gamma-1} - k_{\gamma-2})^\top}{\mu_{\gamma-2}} (\eta_\gamma - k_{\gamma-1} + k_{\gamma-1} \\ &\qquad \qquad \qquad \qquad \qquad \quad - \sum_{s=1}^{\gamma-2} \frac{\partial k_{\gamma-2}}{\partial \eta_s} \dot{\eta}_s) \\
    &-\frac{(\eta_\gamma - k_{\gamma-1})^\top}{\mu_{\gamma-1}} (F+G k_u - \sum_{s=1}^{\gamma-1} \frac{\partial k_{\gamma-1}}{\eta_s} \dot{\eta}_s)
\end{align*}

By rearranging the corresponding terms, 

\begin{align*}
    \dot{\psi_\gamma}(\bm{y}) =& (\frac{\partial \psi(y)}{\partial y})^\top k_1 + (\eta_2 - k_1)^\top \frac{\partial \psi(y)}{\partial y} \\
    &- \frac{(\eta_2 - k_1)^\top}{\mu_1} (k_2 - \sum_{s=1}^1 \frac{\partial k_1}{\partial \eta_s} \dot{\eta}_s) - (\eta_3 - k_2)^\top \frac{\eta_2 - k_1}{\mu_1} \\
    &- \frac{(\eta_3-k_2)^\top}{\mu_2}(k_3 - \sum_{s=1}^2 \frac{\partial k_2}{\partial \eta_s} \dot{\eta}_s) - (\eta_4 - k_3)^\top \frac{\eta_3-k_2}{\mu_2} \\
    & \cdots \\
    &- \frac{(\eta_{\gamma-2} - k_{\gamma-3})^\top}{\mu_{\gamma-3}} (k_{\gamma-2} - \sum_{s=1}^{\gamma-3} \frac{\partial k_{\gamma-3}}{\partial \eta_s} \dot{\eta}_s) \\
    & \qquad \qquad \qquad \qquad \quad  - (\eta_{\gamma-1} - k_{\gamma-2})^\top \frac{\eta_{\gamma-2}- k_{\gamma-3}}{\mu_{\gamma-3}} \\
    &- \frac{(\eta_{\gamma-1} - k_{\gamma-2})^\top}{\mu_{\gamma-2}} (k_{\gamma-1} - \sum_{s=1}^{\gamma-2} \frac{\partial k_{\gamma-2}}{\partial \eta_s} \dot{\eta}_s)) \\
    & \qquad \qquad \qquad \qquad \quad - (\eta_\gamma - k_{\gamma-1})^\top \frac{\eta_{\gamma-1} - k_{\gamma-2}}{\mu_{\gamma-2}} \\
    &-\frac{(\eta_\gamma - k_{\gamma-1})^\top}{\mu_{\gamma-1}} (F+G k_u - \sum_{s=1}^{\gamma-1} \frac{\partial k_{\gamma-1}}{\eta_s} \dot{\eta}_s) \\
    =& (\frac{\partial \psi(y)}{\partial y})^\top k_1 \\
    &- (\eta_2 - k_1)^\top 
    \bigg[ 
        - \frac{\partial \psi(y)}{\partial y} + \frac{k_2 - \sum_{s=1}^1 \frac{\partial k_1}{\partial \eta_s} \dot{\eta}_s}{\mu_1} 
    \bigg] \\
    & - (\eta_3 - k_2)^\top 
    \bigg[
        \frac{\eta_2 - k_1}{\mu_1} + \frac{k_3 - \sum_{s=1}^2 \frac{\partial k_2}{\partial \eta_s} \dot{\eta}_s}{\mu_2}
    \bigg] \\
    & \cdots \\
    &- (\eta_{\gamma-1} - k_{\gamma-2})^\top
    \bigg[
        \frac{\eta_{\gamma-2}- k_{\gamma-3}}{\mu_{\gamma-3}} + \frac{k_{\gamma-1} - \sum_{s=1}^{\gamma-2} \frac{\partial k_{\gamma-2}}{\partial \eta_s} \dot{\eta}_s)}{\mu_{\gamma-2}} 
    \bigg] \\
    &- (\eta_\gamma - k_{\gamma-1})^\top
    \bigg[
        \frac{\eta_{\gamma-1} - k_{\gamma-2}}{\mu_{\gamma-2}} + \frac{F+G k_u - \sum_{s=1}^{\gamma-1} \frac{\partial k_{\gamma-1}}{\eta_s} \dot{\eta}_s}{\mu_{\gamma-1}}
    \bigg]
\end{align*}

For $k_2$,

\begin{align*}
    \frac{\lambda(\eta_2 - k_1)}{2\mu_1} &= - \frac{\partial \psi(y)}{\partial y} + \frac{k_2 - \sum_{s=1}^1 \frac{\partial k_1}{\partial \eta_s} \dot{\eta}_s}{\mu_1}  \\
    \frac{\lambda}{2} (\eta_2 - k_1) &= - \mu_1 \frac{\partial \psi(y)}{\partial y} + k_2 - \sum_{s=1}^1 \frac{\partial k_1}{\partial \eta_s} \\
    k_2 &= \mu_1 \frac{\partial \psi(y)}{\partial y} + \frac{\lambda}{2} (\eta_2 - k_1) + \sum_{s=1}^1 \frac{\partial k_1}{\partial \eta_s}
\end{align*}

For $k_i, i \in \{3, \cdots, \gamma-1\}$,

\begin{align*}
    \frac{\lambda}{2 \mu_{i-1}} (\eta_i - k_{i-1}) = \frac{\eta_{i-1} - k_{i-2}}{\mu_{i-2}} + \frac{k_i - \sum_{s=1}^{i-1} \frac{\partial k_{i-1}}{\partial \eta_s} \dot{\eta}_s}{\mu_{i-1}} \\
    \frac{\lambda}{2} (\eta_i - k_{i-1}) = \frac{\mu_{i-1}(\eta_{i-1} - k_{i-2})}{\mu_{i-1}} + k_i - \sum_{s=1}^{i-1} \frac{\partial k_{i-1}}{\partial \eta_s} \dot{\eta}_s \\
    k_i = - \frac{\mu_{i-1}(\eta_{i-1} - k_{i-2})}{\mu_{i-1}} + \sum_{s=1}^{i-1} \frac{\partial k_{i-1}}{\partial \eta_s} \dot{\eta}_s + \frac{\lambda}{2} (\eta_i - k_{i-1})
\end{align*}

For $k_u$,
\begin{align*}
    \frac{\lambda(\eta_\gamma - k_{\gamma-1})}{2 \mu_{\gamma-1}} = \frac{\eta_{\gamma-1} - k_{\gamma-2}}{\mu_{\gamma-2}} + \frac{F+G k_u - \sum_{s=1}^{\gamma-1} \frac{\partial k_{\gamma-1}}{\eta_s} \dot{\eta}_s}{\mu_{\gamma-1}} \\
    \frac{\lambda}{2} (\eta_\gamma - k_{\gamma-1}) = \frac{\mu_{\gamma-1}(\eta_{\gamma-1} - k_{\gamma-2})}{\mu_{\gamma-2}} + F+G k_u - \sum_{s=1}^{\gamma-1} \frac{\partial k_{\gamma-1}}{\eta_s} \dot{\eta}_s \\
    k_u = G^\dagger 
    \bigg[
        -F - \frac{\mu_{\gamma-1}(\eta_{\gamma-1} - k_{\gamma-2})}{\mu_{\gamma-2}}  + \sum_{s=1}^{\gamma-1} \frac{\partial k_{\gamma-1}}{\eta_s} \dot{\eta}_s  + \frac{\lambda}{2} (\eta_\gamma - k_{\gamma-1})
    \bigg]
\end{align*}

\subsection{Proof of Theorem 2}

Given 
\begin{align}
    \psi_\gamma(x) = \psi(y(x)) - \sum_{i=1}^m \sum_{l=1}^{\gamma_i -1} \frac{1}{2\mu_l} \| \eta_{l+1}^i - k_l^i(z_l^i) \|_2^2
\end{align}

Take the derivative of $\psi_\gamma(x)$ with respect to time,
\begin{align}
    \dot{\psi}_{\gamma}(x) =& \frac{\partial \psi}{\partial y} \dot{y} 
    - \sum_{i=1}^m \sum_{l=1}^{\gamma_i -1} \frac{1}{\mu_l^i} (\eta_{l+1}^i - k_l^i(z_l^i))^\top (\dot{\eta}_{l+1}^i - \sum_{s=1}^l \frac{\partial k_l^i}{\partial \eta_s^i} \dot{\eta}_s^i) \\
    =& \sum_{i=1}^m \frac{\partial \psi}{\partial y_i} \dot{y}_i 
    - \sum_{i=1}^m \sum_{l=1}^{\gamma_i -1} \frac{1}{\mu_l^i} (\eta_{l+1}^i - k_l^i(z_l^i))^\top (\dot{\eta}_{l+1}^i - \sum_{s=1}^l \frac{\partial k_l^i}{\partial \eta_s^i} \dot{\eta}_s^i) \\
    =& \sum_{i=1}^m \bigg[
    \frac{\partial \psi}{\partial y_i} \dot{y}_i - \sum_{l=1}^{\gamma_i -1} \frac{1}{\mu_l^i} (\eta_{l+1}^i - k_l^i(z_l^i))^\top (\dot{\eta}_{l+1}^i - \sum_{s=1}^l \frac{\partial k_l^i}{\partial \eta_s^i} \dot{\eta}_s^i) 
    \bigg] \\
    =& \sum_{i=1}^m \bigg[
    \frac{\partial \psi}{\partial y_i} (\dot{y}_i + k_1^i(y) -  k_1^i(y)) - ...
    \bigg]
\end{align}
